# Supplementary material for: Parameter Estimation and Identifiability in Kinetic Flux Profiling Models of Metabolism
Source: arXiv:2407.08844 source file (2024-07-11)
Supplement: Supplementary file 1 [file supplementary_file_1.pdf]

# 1 Steady-State Problem - Supplementary Information

## 1.1 Irreversible Two-Metabolite Similar Turnover Rates Example

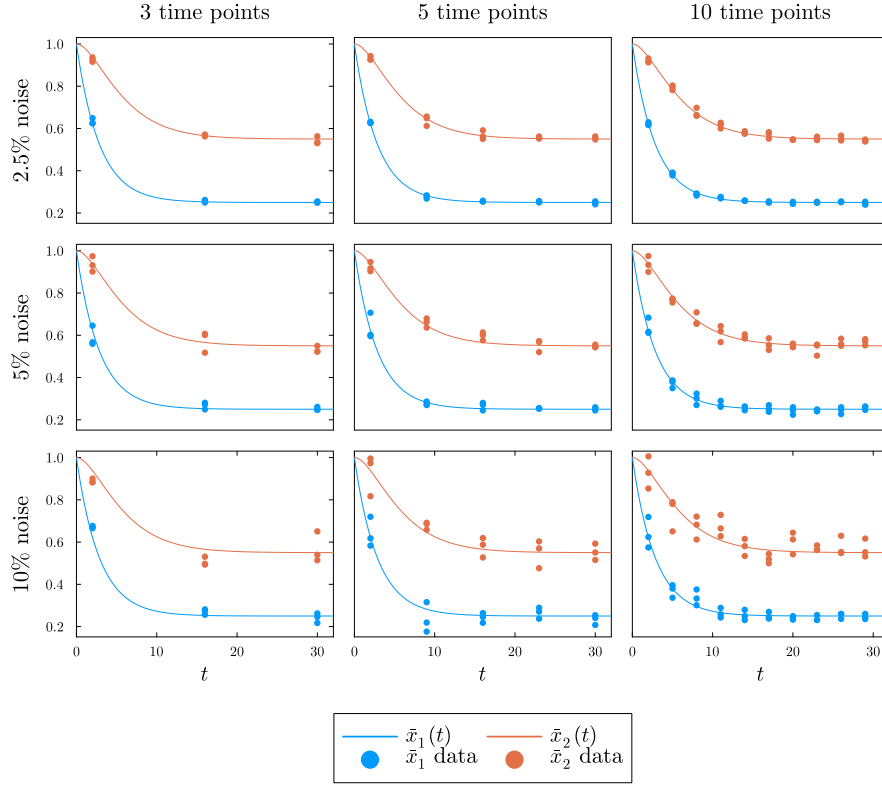

**Fig. 1** Solutions and simulated noisy data for the irreversible two-metabolite model with similar turnover rates. The simulated data are taken from solutions of the system with parameters  $k_1 = 7/20$ ,  $\alpha_1 = 1/4$ ,  $k_2 = 3/10$ ,  $\alpha_2 = 2/5$  at 3, 5 or 10 equally distributed time points. At each time point, three noisy data points are simulated by adding random normally distributed noise to the true solutions with a standard deviation of 2.5, 5, or 10% of the true value

In fig. 1, we see that the experimental measurements are taken while both  $\bar{x}_1$  and  $\bar{x}_2$  are still decaying and as both approach their steady-state values. Since the experimental data captures information about the decay rates and steady-state values we expect to get accurate estimates of all parameter values with low uncertainty given sufficient time points and little noise.

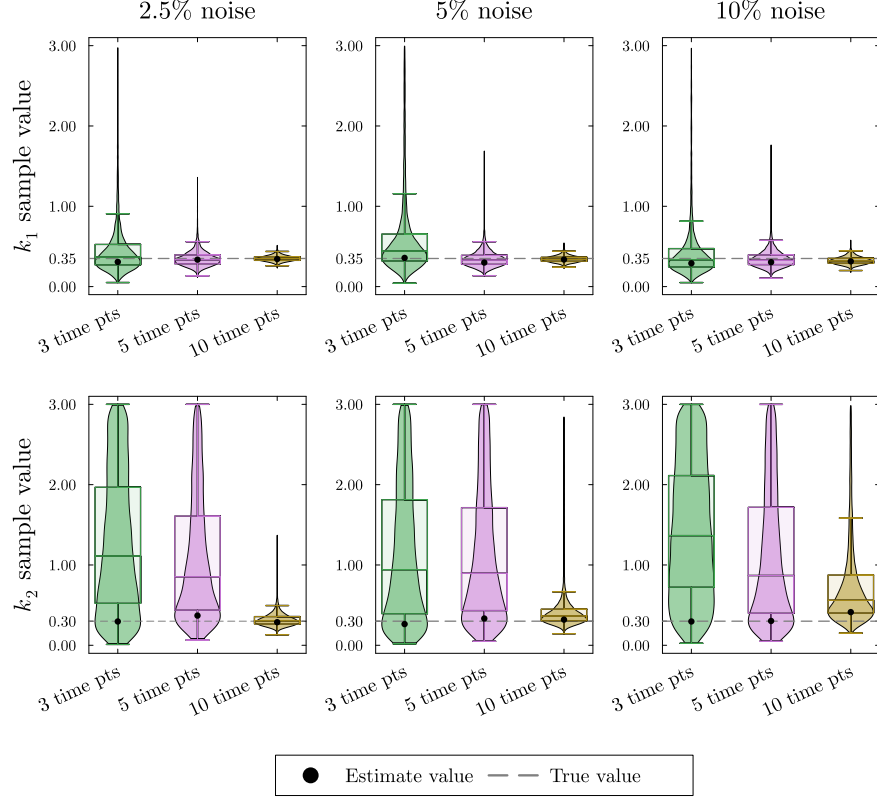

**Fig. 2** Violin and box plots for posterior distributions of  $k_1$  and  $k_2$  for the irreversible two-metabolite model with similar turnover rates. The simulated data are taken from solutions of the system with parameters  $k_1 = 7/20$ ,  $\alpha_1 = 1/4$ ,  $k_2 = 3/10$ ,  $\alpha_2 = 2/5$  at 3, 5 or 10 equally distributed time points. At each time point, three noisy data points are simulated by adding random normally distributed noise to the true solutions with a standard deviation of 2.5, 5, or 10% of the true value. Since  $k_1$ ,  $k_2$  and  $k_3$  are turnover rates, we use the naive prior distributions  $k_1 \sim U(0, 3)$ ,  $k_2 \sim U(0, 3)$ . The mode of the posterior samples is taken as the estimated value. Outliers are excluded in the box plots

From fig. 2, we see that the Bayesian estimation method condensed the sample values near the true parameter values for both parameters. Regardless of the noise level, the parameter estimation increases in accuracy with the inclusion of more time points. The estimated value of the posterior distributions approaches the true parameter value as the number of time points increases. We also note that the uncertainty in the estimation decreases with the increase in time points. With 10 time points and 2.5% noise, we receive the best estimates with the least uncertainty for both  $k_1$  and  $k_2$ .

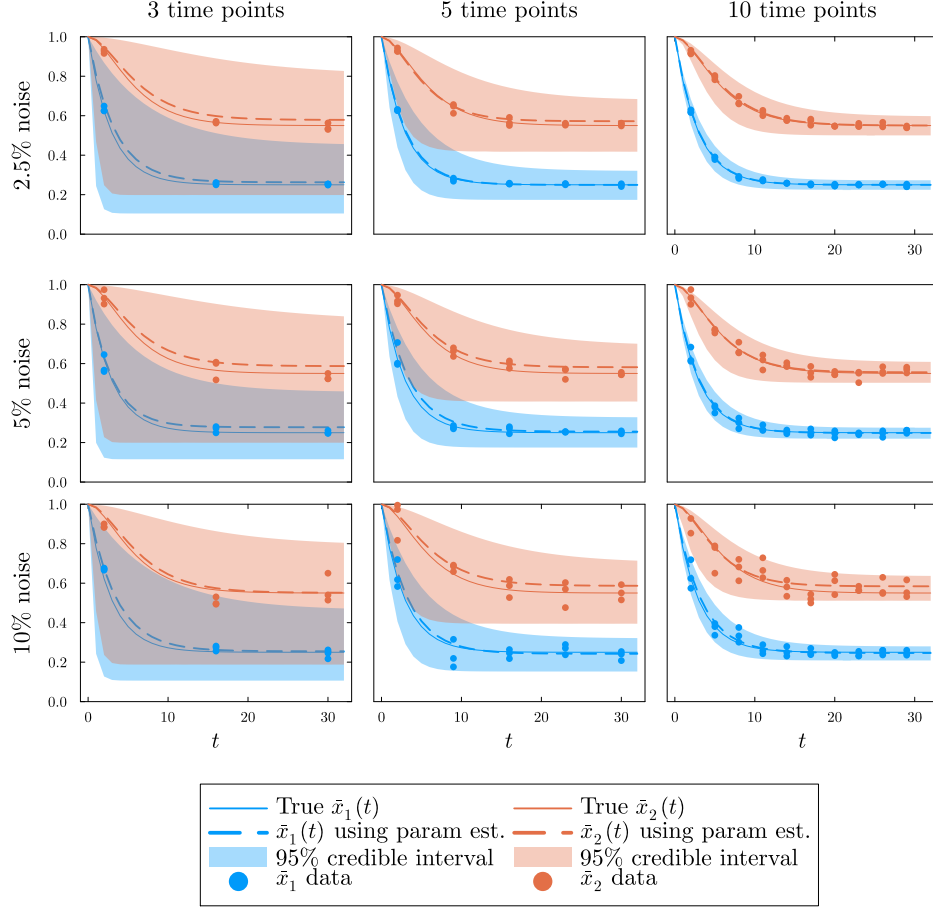

**Fig. 3** Comparing solutions using the values produced from Bayesian parameter estimation to the experimental data and true solutions for the irreversible two-metabolite model with similar turnover rates. The simulated data are taken from solutions of the system with parameters  $k_1 = 7/20$ ,  $\alpha_1 = 1/4$ ,  $k_2 = 3/10$ ,  $\alpha_2 = 2/5$  at 3, 5 or 10 equally distributed time points. At each time point, three noisy data points are simulated by adding random normally distributed noise to the true solutions with a standard deviation of 2.5, 5, or 10% of the true value. The 95% credible interval was created by plotting the region between the solution with the 2.5% and the 97.5% quartiles of the posterior distributions of the parameters

In fig. 3, we see that the solution using the parameter estimates approaches the true solution as we increase the number of time points. The 95% credible interval is the region where 95% trajectories produced by the samples from the posterior parameter distributions would be. Also, the 95% credible interval tightens around the true solution as we increase the number of time points and decrease the level of noise in the measurements.

## 1.2 Reversible Two-Metabolite Similar Turnover Rates Example

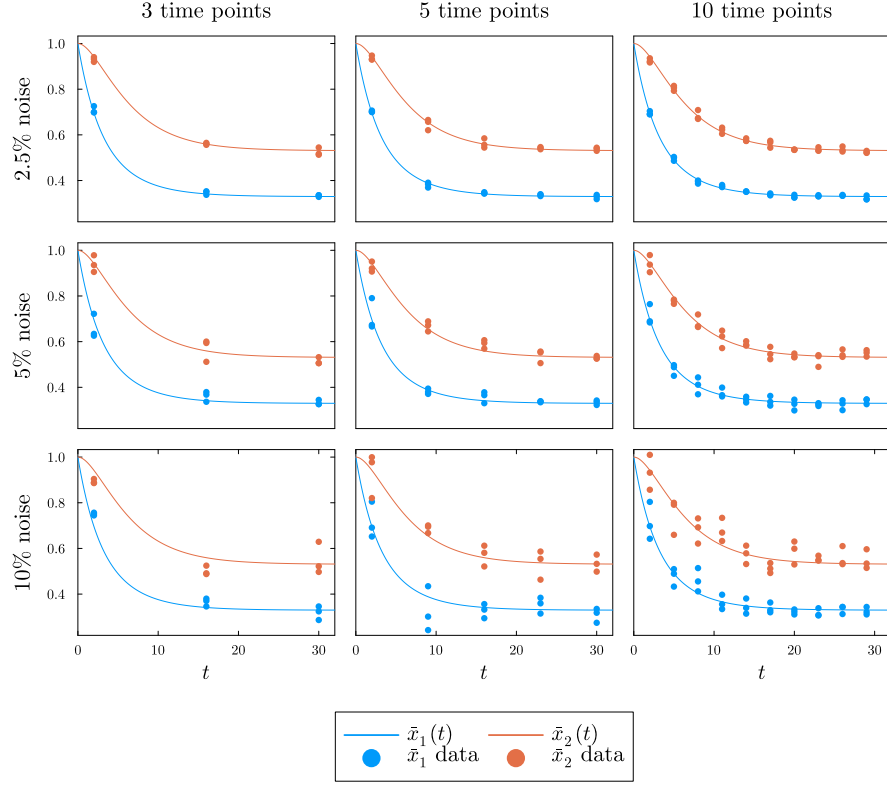

**Fig. 4** Solutions and simulated noisy data for the reversible two-metabolite model with similar turnover rates. The simulated data are taken from solutions of the system with parameters  $k_1 = 7/20$ ,  $\alpha_1 = 3/10$ ,  $\beta_{2,1} = 3/20$ ,  $k_2 = 3/10$ ,  $\alpha_2 = 1/4$  at 3, 5 or 10 equally distributed time points. At each time point, three noisy data points are simulated by adding random normally distributed noise to the true solutions with a standard deviation of 2.5, 5, or 10% of the true value

In fig. 4, we see that the experimental measurements are taken while both  $\bar{x}_1$  and  $\bar{x}_2$  are still decaying and as both approach their steady-state values. Since the experimental data captures information about the decay rates and steady-state values, we expect to get accurate estimates of all parameter values with low uncertainty given sufficient time points and little noise.

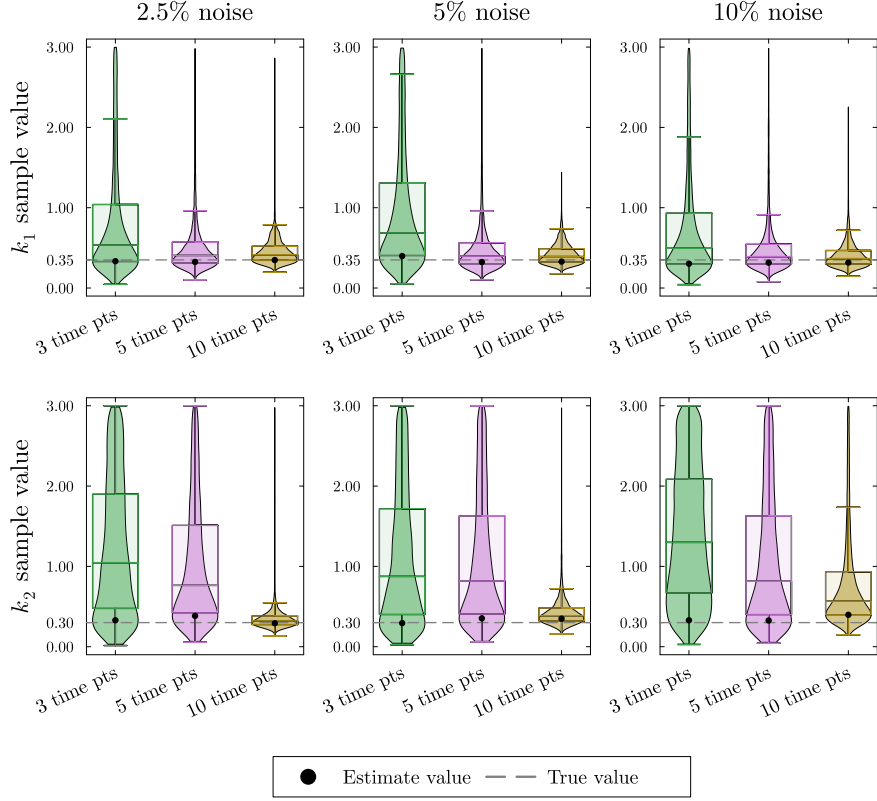

**Fig. 5** Violin and box plots for posterior distributions of  $k_1$  and  $k_2$  for the reversible two-metabolite model with similar turnover rates. The simulated data are taken from solutions of the system with parameters  $k_1 = 7/20$ ,  $\alpha_1 = 3/10$ ,  $\beta_{2,1} = 3/20$ ,  $k_2 = 3/10$ ,  $\alpha_2 = 1/4$  at 3, 5 or 10 equally distributed time points. At each time point, three noisy data points are simulated by adding random normally distributed noise to the true solutions with a standard deviation of 2.5, 5, or 10% of the true value. Since  $k_1$  and  $k_2$  are turnover rates, we use the naive prior distributions  $k_1 \sim U(0, 3)$ ,  $k_2 \sim U(0, 3)$ . The mode of the posterior samples is taken as the estimated value. Outliers are excluded in the box plots.

From fig. 5, we see that the Bayesian estimation method condensed the sample values near the true parameter values for both parameters. Regardless of the noise level, the parameter estimation increases in accuracy with the inclusion of more time points. The estimated value of the posterior distributions approaches the true parameter value as the number of time points increases. With 10 time points and 2.5% noise, we receive the best estimates with the least uncertainty for both  $k_1$  and  $k_2$ .

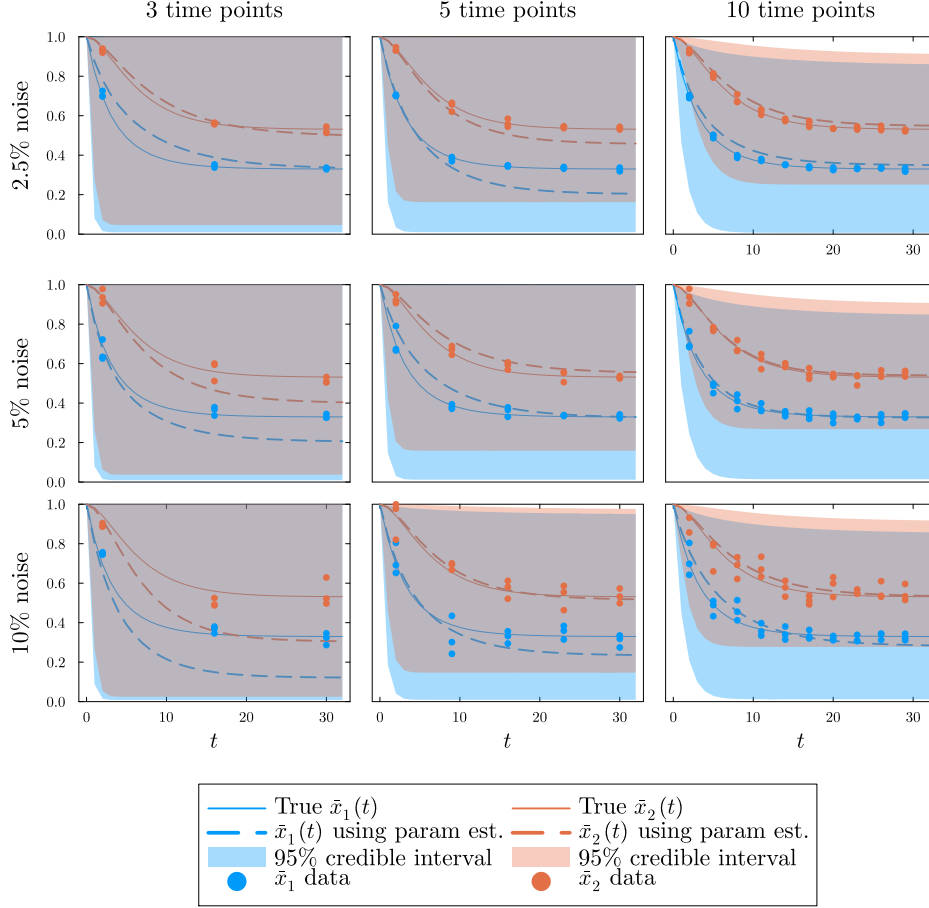

**Fig. 6** Comparing solutions using the values produced from Bayesian parameter estimation to the experimental data and true solutions for the reversible two-metabolite model with similar turnover rates. The simulated data are taken from solutions of the system with parameters  $k_1 = 7/20$ ,  $\alpha_1 = 3/10$ ,  $\beta_{2,1} = 3/20$ ,  $k_2 = 3/10$ ,  $\alpha_2 = 1/4$  at 3, 5 or 10 equally distributed time points. At each time point, three noisy data points are simulated by adding random normally distributed noise to the true solutions with a standard deviation of 2.5, 5, or 10% of the true value. The 95% credible interval was created by plotting the region between the solution with the 2.5% and the 97.5% quartiles of the posterior distributions of the parameters

In fig. 6, we see that the solution using the parameter estimates approaches the true solution as we increase the number of time points. The 95% credible interval does not decrease much due to the high uncertainty in the parameter values. Given many time points, it appears that the method is accurately estimating the steady-state values for  $\bar{x}_1$  and  $\bar{x}_2$  while inaccurately estimating the true values of  $\alpha_1$  and  $\beta_{1,2}$ .

## 2 Fast-Slow Analysis - Supplementary Information

### 2.1 Reversible Two-Metabolite Fast-Slow Example

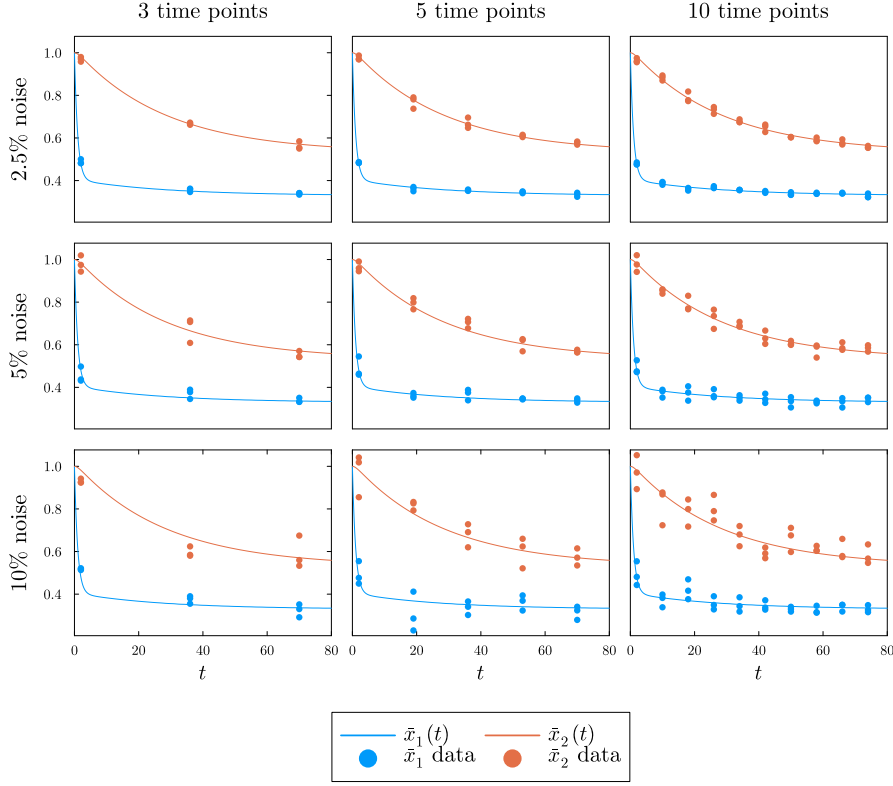

**Fig. 7** Solutions and simulated noisy data for the reversible two-metabolite model with similar turnover rates. The simulated data are taken from solutions of the system with parameters  $k_1 = 1$ ,  $\alpha_1 = 1/4$ ,  $\beta_{1,2} = 3/20$ ,  $k_2 = 1/25$ ,  $\alpha_2 = 3/10$  at 3, 5 or 10 equally distributed time points. At each time point, three noisy data points are simulated by adding random normally distributed noise to the true solutions with a standard deviation of 2.5, 5, or 10% of the true value

In fig. 7, we see that most of the experimental measurements are taken while  $\bar{x}_1$  is near its steady-state value and  $\bar{x}_2$  is still decaying. Only one of the time points is taken while  $\bar{x}_1$  rapidly decays immediately after the isotope switch. Also, the time frame of the measurements does not extend far enough to truly capture  $\bar{x}_2$  near its steady-state value.

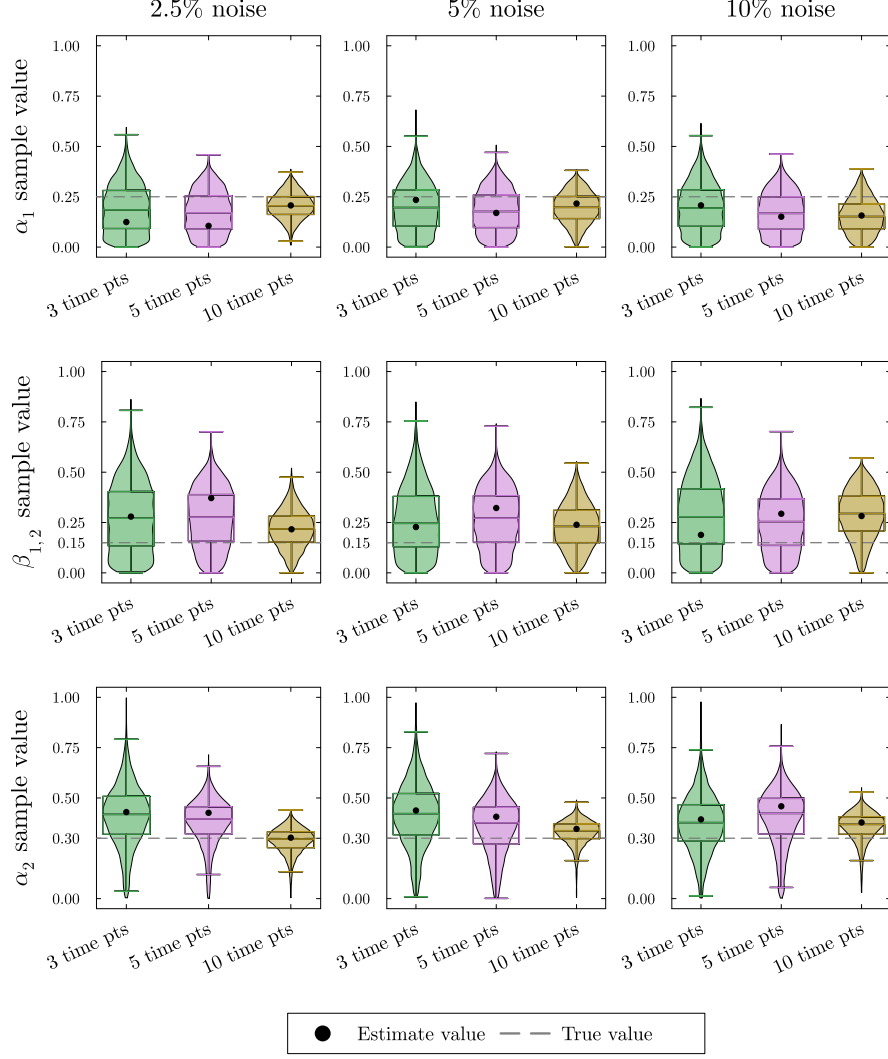

**Fig. 8** Violin and box plots for posterior distributions of  $\alpha_1$ ,  $\beta_{1,2}$ , and  $\alpha_2$  for the reversible two-metabolite fast-slow system. The simulated data are taken from solutions of the system with parameters  $k_1 = 1$ ,  $\alpha_1 = 1/4$ ,  $\beta_{1,2} = 3/20$ ,  $k_2 = 1/25$ ,  $\alpha_2 = 3/10$  at 3, 5 or 10 equally distributed time points. At each time point, three noisy data points are simulated by adding random normally distributed noise to the true solutions with a standard deviation of 2.5, 5, or 10% of the true value. Since  $\alpha_1$ ,  $\beta_{1,2}$ , and  $\alpha_2$  are proportions, we use the natural naive prior distributions  $\alpha_1 \sim U(0,1)$ ,  $\beta_{1,2} \sim U(0,1)$ , and  $\alpha_2 \sim U(0,1)$ . The mode of the posterior samples is shown as a dot and is taken as the estimated value. Outliers are excluded in the box plots

As expected, in fig. 11, we get poor estimates with high uncertainty for  $\alpha_1$  and  $\beta_{1,2}$ . On the bottom row of fig. 8, we see that increasing the number of time points



produces a more accurate estimate for  $\alpha_2$ . We also note that the uncertainty in the estimation decreases with the increase in time points.

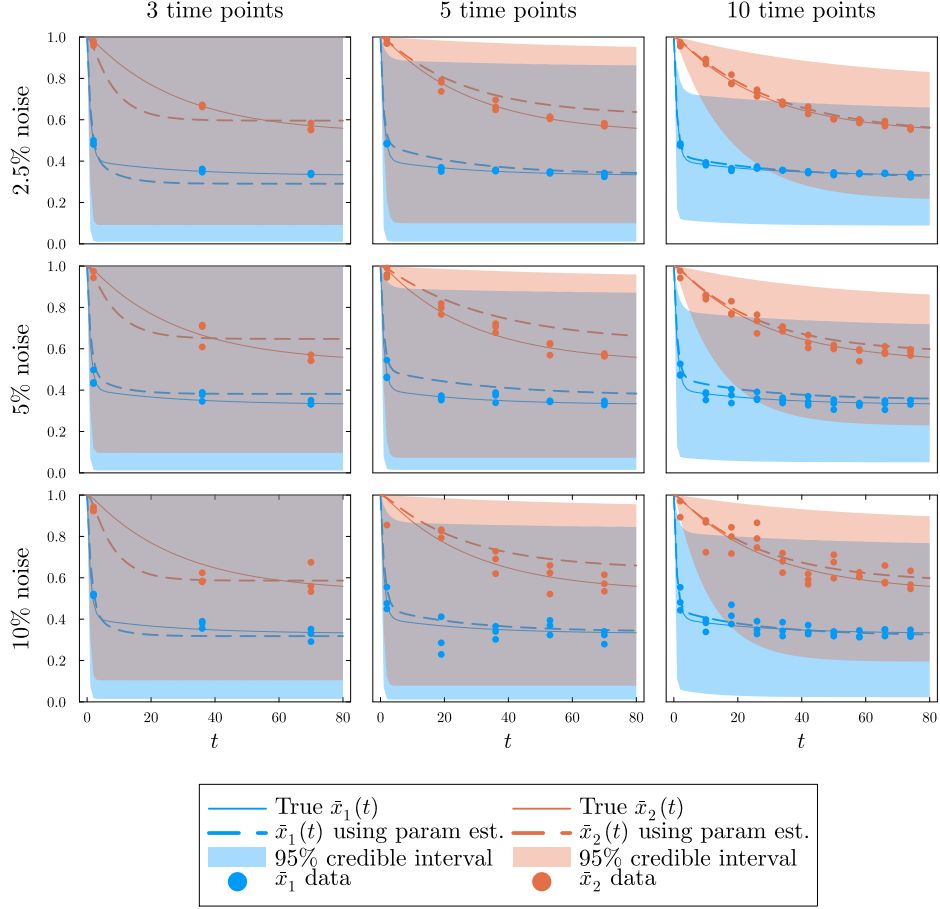

**Fig. 9** Comparing solutions using the values produced from Bayesian parameter estimation to the experimental data and true solutions for the reversible two-metabolite model with similar turnover rates. The simulated data are taken from solutions of the system with parameters  $k_1 = 1$ ,  $\alpha_1 = 1/4$ ,  $\beta_{1,2} = 3/20$ ,  $k_2 = 1/25$ ,  $\alpha_2 = 3/10$  at 3, 5 or 10 equally distributed time points. At each time point, three noisy data points are simulated by adding random normally distributed noise to the true solutions with a standard deviation of 2.5, 5, or 10% of the true value. The 95% credible interval was created by plotting the region between the solution with the 2.5% and the 97.5% quartiles of the posterior distributions of the parameters

In fig. 9, we see that the solution using the parameter estimates approaches the true solution as we increase the number of time points. Again, the 95% credible interval does not decrease much due to the high uncertainty in the parameter values. Given many time points and minimal noise, it appears that the method is accurately estimating

the steady-state values for  $\bar{x}_1$  and  $\bar{x}_2$  while inaccurately estimating the true values of  $\alpha_1$  and  $\beta_{1,2}$ .

## 2.2 Reversible Two-Metabolite Slow-Fast Example

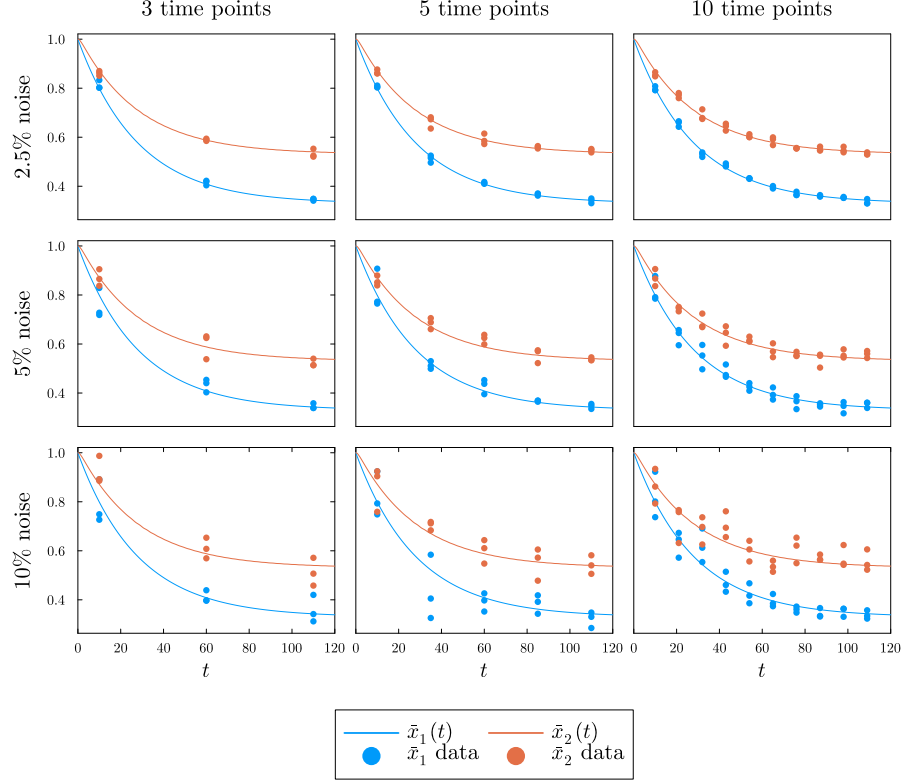

**Fig. 10** Solutions and simulated noisy data for the reversible two-metabolite slow-fast system. The simulated data are taken from solutions of the system with parameters  $k_1 = 1/25$ ,  $\alpha_1 = 1/4$ ,  $\beta_{1,2} = 3/20$ ,  $k_2 = 1$ ,  $\alpha_2 = 3/10$  at 3, 5 or 10 equally distributed time points. At each time point, three noisy data points are simulated by adding random normally distributed noise to the true solutions with a standard deviation of 2.5, 5, or 10% of the true value

In fig. 10, we see that the experimental measurements are taken while both  $\bar{x}_1$  and  $\bar{x}_2$  are still decaying and as both approach their steady-state values. In this case, we know that experimental measurements of  $\bar{x}_2$  do not contain fast dynamics because the initial condition of the experiment is on the slow manifold.

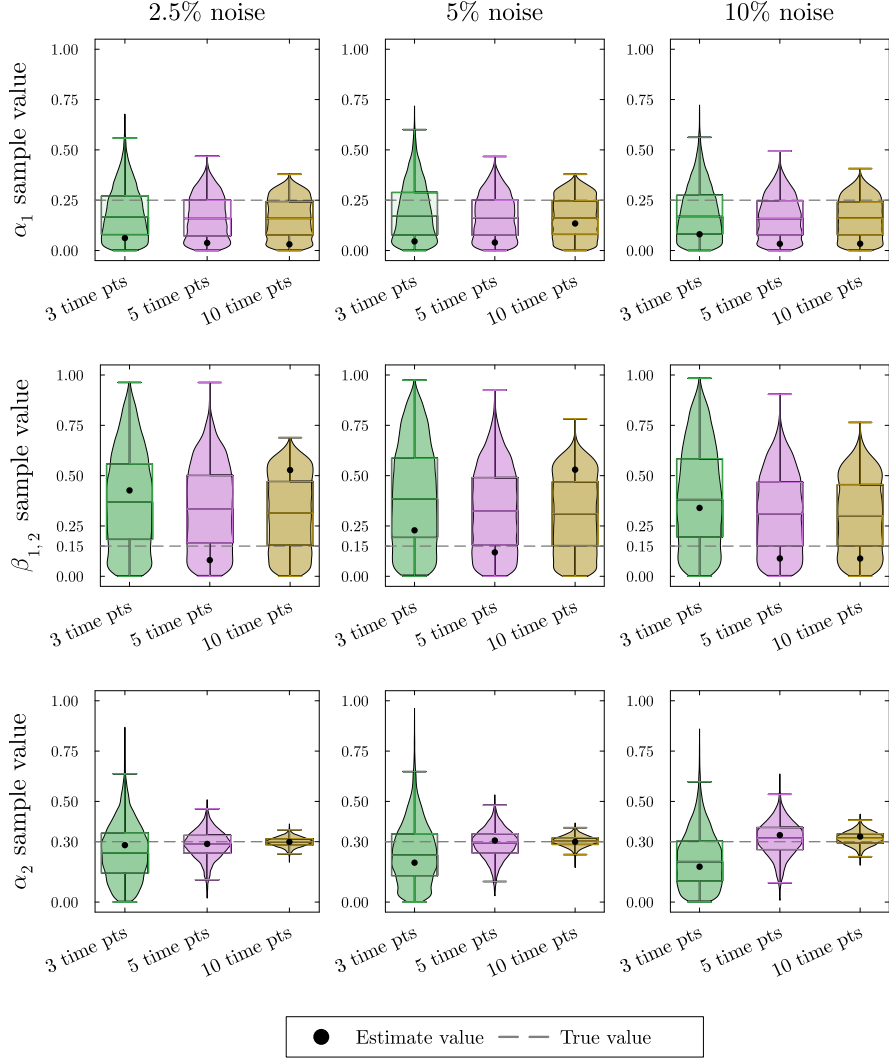

**Fig. 11** Violin and box plots for posterior distributions of  $\alpha_1$ ,  $\beta_{1,2}$ , and  $\alpha_2$  for the reversible two-metabolite fast-slow system. The simulated data are taken from solutions of the system with parameters  $k_1 = 1$ ,  $\alpha_1 = 1/4$ ,  $\beta_{1,2} = 3/20$ ,  $k_2 = 1/25$ ,  $\alpha_2 = 3/10$  at 3, 5 or 10 equally distributed time points. At each time point, three noisy data points are simulated by adding random normally distributed noise to the true solutions with a standard deviation of 2.5, 5, or 10% of the true value. Since  $\alpha_1$ ,  $\beta_{2,1}$ , and  $\alpha_2$  are proportions, we use the natural naive prior distributions  $\alpha_1 \sim U(0, 1)$ ,  $\beta_{2,1} \sim U(0, 1)$ , and  $\alpha_2 \sim U(0, 1)$ . The mode of the posterior samples is shown as a dot and is taken as the estimated value. Outliers are excluded in the box plots

As expected, in fig. 11, we get poor estimates with high uncertainty for  $\alpha_1$  and  $\beta_{1,2}$ . On the bottom row of fig. 11, we see that increasing the number of time points

produces a more accurate estimate for  $\alpha_2$ . We also note that the uncertainty in the estimation decreases with the increase in time points.

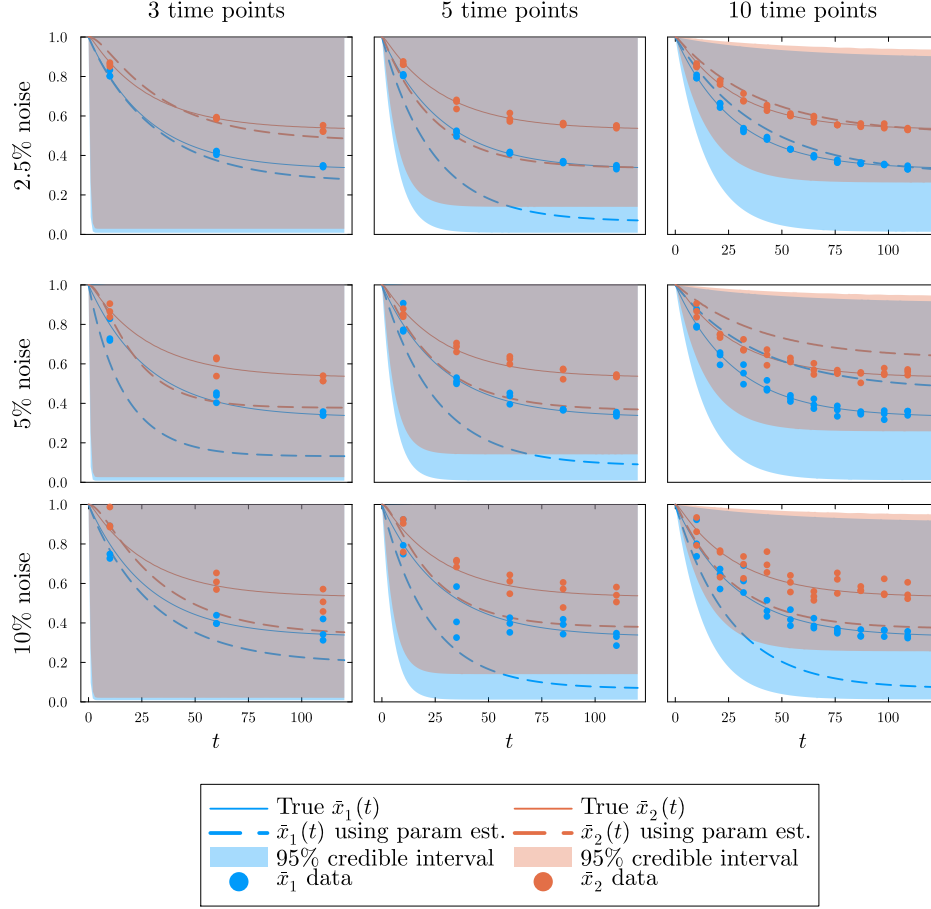

**Fig. 12** Comparing solutions using the values produced from Bayesian parameter estimation to the experimental data and true solutions for the reversible two-metabolite slow-fast system. The simulated data are taken from solutions of the system with parameters  $k_1 = 1/25$ ,  $\alpha_1 = 1/4$ ,  $\beta_{1,2} = 3/10$ ,  $k_2 = 1$ ,  $\alpha_2 = 3/10$  at 3, 5 or 10 equally distributed time points. At each time point, three noisy data points are simulated by adding random normally distributed noise to the true solutions with a standard deviation of 2.5, 5, or 10% of the true value. The 95% credible interval was created by plotting the region between the solution with the 2.5% and the 97.5% quartiles of the posterior distributions of the parameters

In fig. 12, it appears the inaccuracy and high uncertainty in the estimate for  $k_2$ ,  $\alpha_1$ , and  $\beta_{1,2}$  show in solutions using the estimated parameter values. The 95% credible interval for both  $\bar{x}_1$  and  $\bar{x}_2$  show a large range for possible estimates. Overall, this case produced the worst solutions with the estimated parameter values.

### 2.3 Irreversible Two-Metabolite Fast-Slow Example

Consider the irreversible two-metabolite reaction network. Suppose we know the turnover rate of  $X_1$  is much greater than the turnover rate of  $X_2$ , i.e.  $k_1 \gg k_2$ . Let the dimensionless variables  $\tau = k_1 t$  be the fast time scale and let  $\epsilon = k_2/k_1 \ll 1$  then the fast subsystem is.

$$\begin{aligned}\frac{d\bar{x}_1}{d\tau} &= -\bar{x}_1 + \alpha_1 \\ \bar{x}_2 &= 1\end{aligned}$$

Let  $\eta = \epsilon \tau$  be the slow time scale to obtain the slow subsystem.

$$\begin{aligned}0 &= -\bar{x}_1 + \alpha \\ \frac{d\bar{x}_2}{d\eta} &= (1 - \alpha_2)\bar{x}_1 - \bar{x}_2 + \alpha_2\end{aligned}$$

In this example, the slow manifold is defined by the line  $\bar{x}_1 = \alpha_1$ .

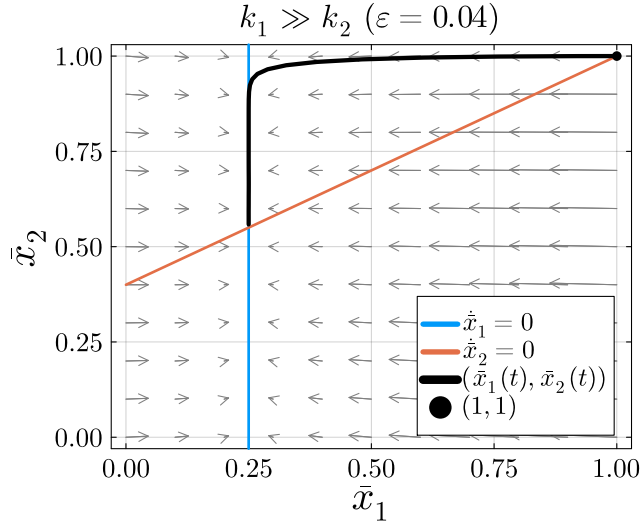

**Fig. 13** The phase plane for the irreversible two-metabolite model in the case where the turnover rate of  $X_1$  is much greater than the turnover rate of  $X_2$ . The parameter values used to create this figure are  $k_1 = 1$ ,  $\alpha_1 = 1/4$ ,  $k_2 = 1/25$ , and  $\alpha_2 = 2/5$

The solution  $(\bar{x}_1(t), \bar{x}_2(t))$  in fig. 13 begins at the initial condition  $(1, 1)$ . Next, it quickly moves from the initial condition toward the slow manifold  $\bar{x}_1 = \alpha_1$ . This portion of the solution shows the fast dynamics of the system. After approaching the line  $\bar{x}_1 = \alpha_1$ , the solution slowly moves towards the equilibrium  $(\alpha_1, \alpha_1 - \alpha_1 \alpha_2 + \alpha_2)$

at the intersection of  $\dot{x}_1 = 0$  and  $\dot{x}_2 = 0$ . The movement along the slow manifold represents the slow dynamics of the system. In this example, data collected quickly after the isotope switch will be on the fast time scale and data collected later in the experiment will be on the slow time scale. With both early and later measurements from this biological system, KFP will provide more accurate estimations given that both fast and slow dynamics are represented.

To demonstrate parameter estimations we simulate data for this scenario as described in the appendix.

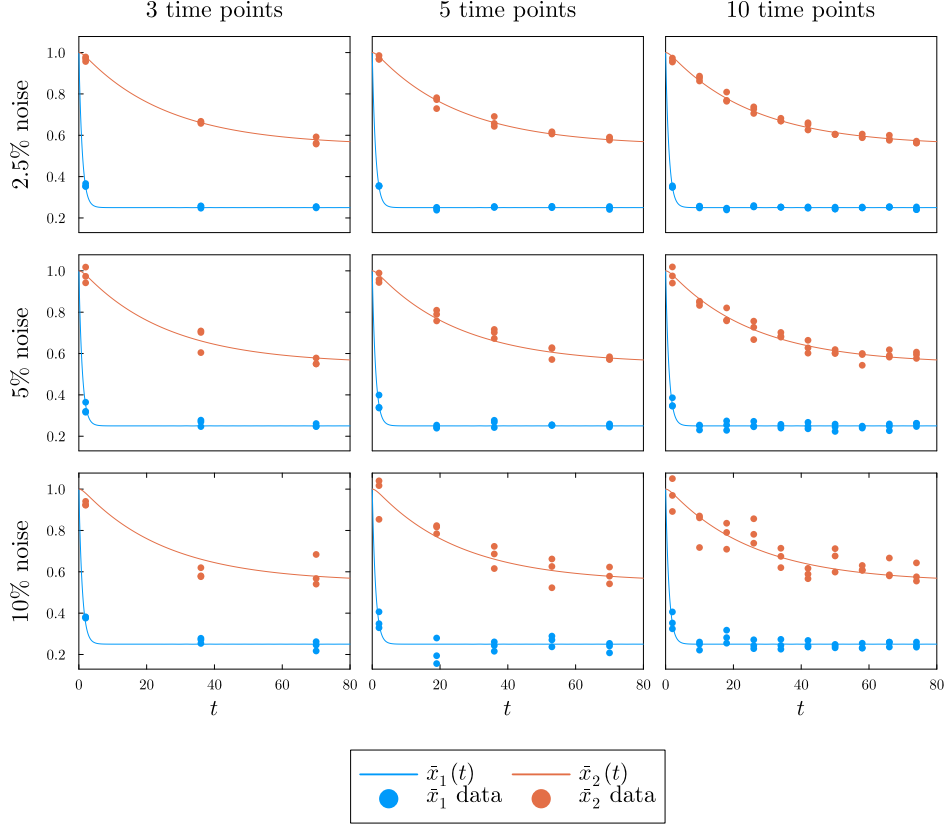

**Fig. 14** Solutions and simulated noisy data for the irreversible two-metabolite fast-slow system. The simulated data are taken from solutions of the system with parameters  $k_1 = 1$ ,  $\alpha_1 = 1/4$ ,  $k_2 = 1/25$ ,  $\alpha_2 = 2/5$  at 3, 5 or 10 equally distributed time points. At each time point, three noisy data points are simulated by adding random normally distributed noise to the true solutions with a standard deviation of 2.5, 5, or 10% of the true value

In fig. 14, we see that most of the experimental measurements are taken while  $\bar{x}_1$  is near its steady-state value, but  $\bar{x}_2$  is still decaying. Only one of the time points is taken while  $\bar{x}_1$  rapidly decays right after the isotope switch. Also, the time frame of

the measurements does not extend far enough to truly capture  $\bar{x}_2$  near its steady-state value.

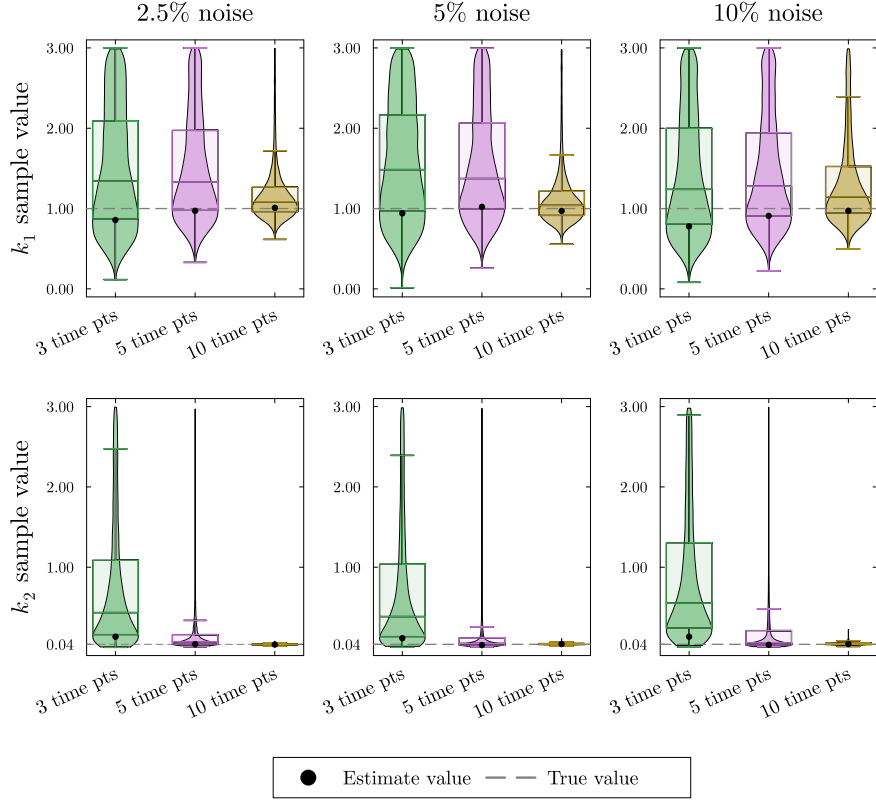

**Fig. 15** Violin and box plots for posterior distributions of  $k_1$  and  $k_2$  for the irreversible two-metabolite fast-slow system. The simulated data are taken from solutions of the system with parameters  $k_1 = 1$ ,  $\alpha_1 = 1/4$ ,  $k_2 = 1/25$ ,  $\alpha_2 = 2/5$  at 3, 5 or 10 equally distributed time points. At each time point, three noisy data points are simulated by adding random normally distributed noise to the true solutions with a standard deviation of 2.5, 5, or 10% of the true value. Since  $k_1$ , and  $k_2$  are turnover rates, we use the naive prior distributions  $k_1 \sim U(0, 3)$ ,  $k_2 \sim U(0, 3)$ . The mode of the posterior samples is taken as the estimated value. Outliers are excluded in the box plots

On the top row of fig. 15, we note that the estimates for  $k_1$  have a large uncertainty. This is because there isn't enough information on the decay rate of  $\bar{x}_1$  in the experimental measurements. With only one of the time points taken during the rapid decay of  $\bar{x}_1$ , we cannot get a good estimate for  $k_1$ . On the bottom row of fig. 15, we see the estimate for  $k_2$  increases in accuracy and decreases in uncertainty with the addition of time points despite the noise level. With 10 time points, the estimate for  $k_2$  is incredibly accurate with very low uncertainty.

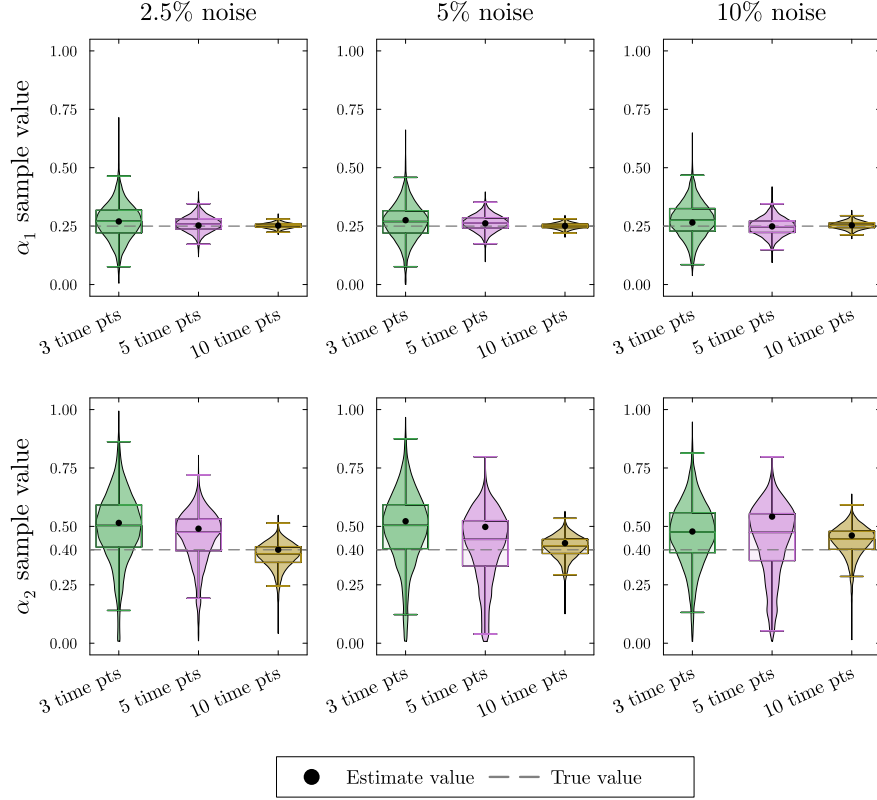

**Fig. 16** Violin and box plots for posterior distributions of  $\alpha_1$  and  $\alpha_2$  for the irreversible two-metabolite fast-slow system. The simulated data are taken from solutions of the system with parameters  $k_1 = 1$ ,  $\alpha_1 = 1/4$ ,  $k_2 = 1/25$ ,  $\alpha_2 = 2/5$  at 3, 5 or 10 equally distributed time points. At each time point, three noisy data points are simulated by adding random normally distributed noise to the true solutions with a standard deviation of 2.5, 5, or 10% of the true value. Since  $\alpha_1$ , and  $\alpha_2$  are proportions, we use the natural naive prior distributions  $\alpha_1 \sim U(0, 1)$ ,  $\alpha_2 \sim U(0, 1)$ . The mode of the posterior samples is shown as a dot and is taken as the estimated value. Outliers are excluded in the box plots

Since many of the experimental measurements are taken while  $\bar{x}_1$  is near steady state, we expected to get an accurate estimate with low uncertainty for  $\alpha_1$  due to its direct relation to  $\bar{x}_1$ 's steady-state. This is clearly shown on the top row of fig. 16. Without experimental measurements of  $\bar{x}_2$  near steady state, we get high uncertainty in the estimates for  $\alpha_2$  as shown on the bottom row of fig. 16. Without the steady-state information for  $\bar{x}_2$ , the Bayesian method estimates the value of  $\alpha_2$  to be higher than its true value.



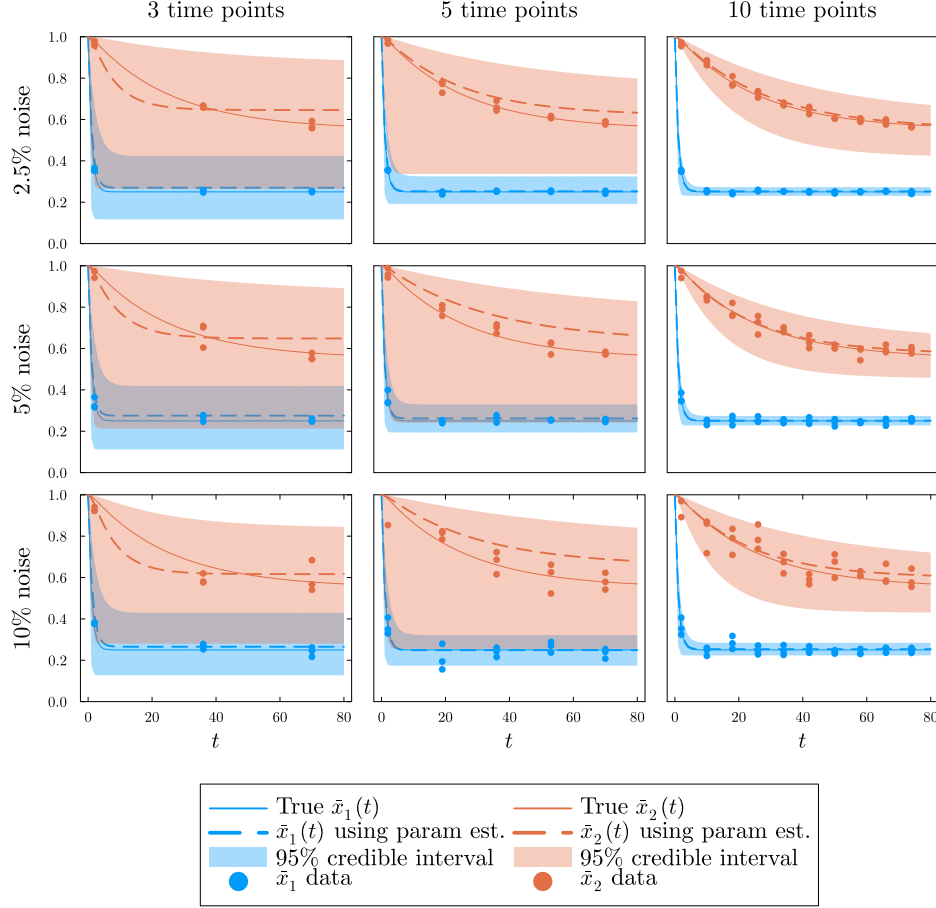

**Fig. 17** Comparing solutions using the values produced from Bayesian parameter estimation to the experimental data and true solutions for the irreversible two-metabolite model fast-slow system. The simulated data are taken from solutions of the system with parameters  $k_1 = 1$ ,  $\alpha_1 = 1/4$ ,  $k_2 = 1/25$ ,  $\alpha_2 = 2/5$  at 3, 5 or 10 equally distributed time points. At each time point, three noisy data points are simulated by adding random normally distributed noise to the true solutions with a standard deviation of 2.5, 5, or 10% of the true value. The 95% credible interval was created by plotting the region between the solution with the 2.5% and the 97.5% quartiles of the posterior distributions of the parameters

In fig. 17, we see that the solution using the parameter estimates approaches the true solution as we increase the number of time points. In this case, the 95% credible interval for  $\bar{x}_1$  does not reflect the inaccuracy and uncertainty in the estimate of  $k_1$ . The solution using the estimated parameter values looks fairly accurate. The inaccuracy and uncertainty is more obvious in the 95% credible interval for  $\bar{x}_2$ .

## 2.4 Irreversible Two-Metabolite Slow-Fast Example

Now, we will assume the opposite situation. Suppose we know the turnover rate of  $X_2$  is much greater than the turnover rate of  $X_1$ , i.e.  $k_2 \gg k_1$ . Let the dimensionless variables  $\tau = k_2 t$  be the fast time scale and let  $\epsilon = k_1/k_2 \ll 1$ . We derive the fast subsystem.

$$\begin{aligned}\bar{x}_1 &= 1 \\ \frac{d\bar{x}_2}{d\tau} &= 1 - \bar{x}_2\end{aligned}$$

Let  $\eta = \epsilon\tau$  be the slow time scale to obtain the slow subsystem.

$$\begin{aligned}\frac{d\bar{x}_1}{d\eta} &= -\bar{x}_1 + \alpha \\ 0 &= (1 - \alpha_2)\bar{x}_1 - \bar{x}_2 + \alpha_2\end{aligned}$$

In this example, the slow manifold is defined by the line  $\bar{x}_2 = (1 - \alpha_2)\bar{x}_1 + \alpha_2$ .

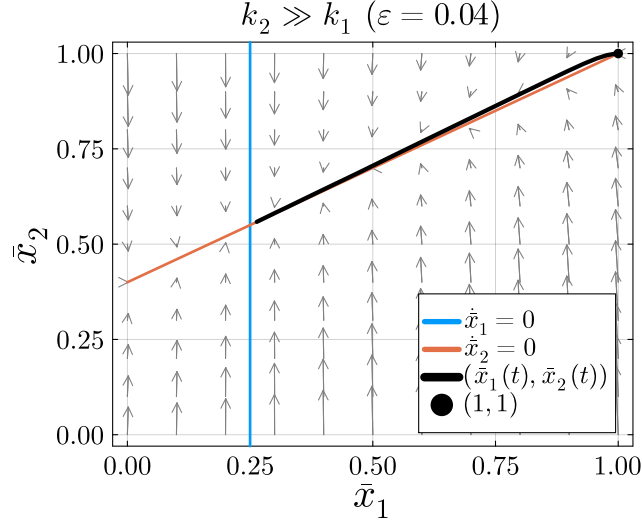

**Fig. 18** The phase plane for the irreversible two-metabolite model in case where the turnover rate of  $X_2$  is much greater than the turnover rate of  $X_1$ . The parameter values used to create this figure are  $k_1 = 1/25$ ,  $\alpha_1 = 1/4$ ,  $k_2 = 1$ , and  $\alpha_2 = 2/5$

The solution  $(\bar{x}_1(t), \bar{x}_2(t))$  in fig. 18 begins at the initial condition  $(1, 1)$ . The initial condition is located on the slow manifold  $\bar{x}_2 = (1 - \alpha_2)\bar{x}_1 + \alpha_2$ . The solution will slowly move along the slow manifold until it approaches the equilibrium  $(\alpha_1, \alpha_1 - \alpha_1\alpha_2 + \alpha_2)$  at the intersection of  $\dot{\bar{x}}_1 = 0$  and  $\dot{\bar{x}}_2 = 0$ . Therefore, only the slow dynamics will

be visible in the experimental data. Metabolite  $X_1$ 's slow turnover rate restricts the amount of label entering metabolite  $X_2$ , preventing an accurate approximation of the much faster rate through  $X_2$ . For the data to display the fast dynamics of  $X_2$ , we would need to change the initial condition of the system. Changing the initial condition would require a different experimental setup.

To demonstrate parameter estimations, we simulate data for this scenario as described in the appendix.

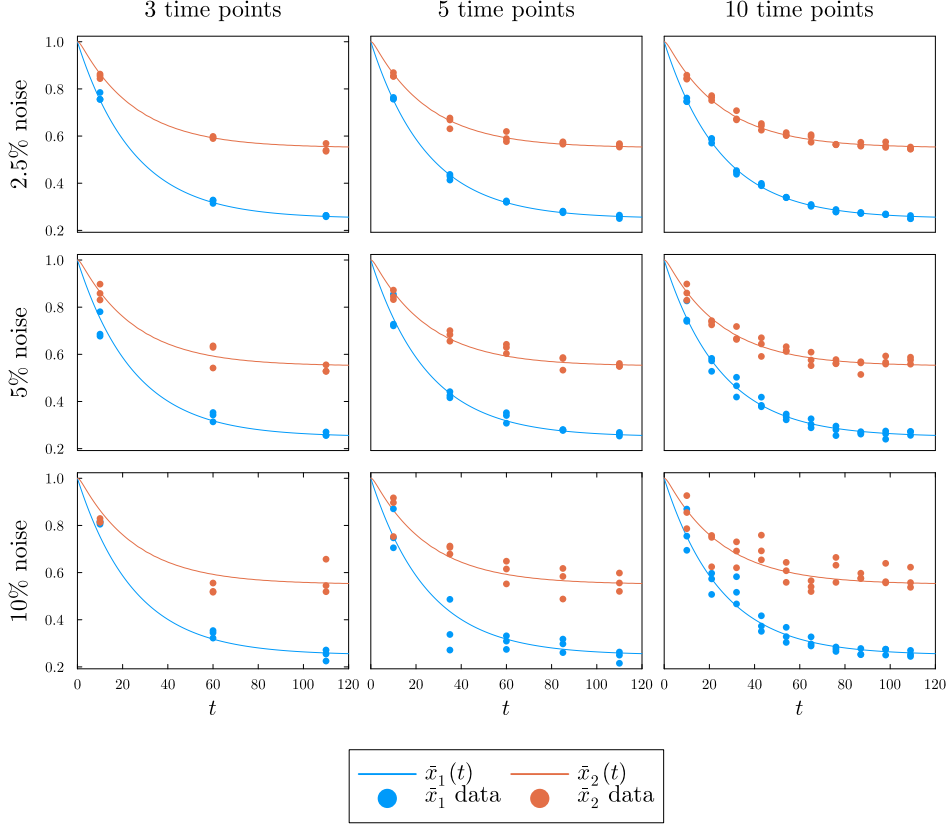

**Fig. 19** Solutions and simulated noisy data for the irreversible two-metabolite slow-fast system. The simulated data are taken from solutions of the system with parameters  $k_1 = 1/25$ ,  $\alpha_1 = 1/4$ ,  $k_2 = 1$ ,  $\alpha_2 = 2/5$  at 3, 5 or 10 equally distributed time points. At each time point, three noisy data points are simulated by adding random normally distributed noise to the true solutions with a standard deviation of 2.5, 5, or 10% of the true value

In fig. 19, we see that the experimental measurements are taken while both  $\bar{x}_1$  and  $\bar{x}_2$  are still decaying and as both approach their steady-state values. In this case, we know that experimental measurements of  $\bar{x}_2$  do not contain fast dynamics because the initial condition of the experiment is on the slow manifold.

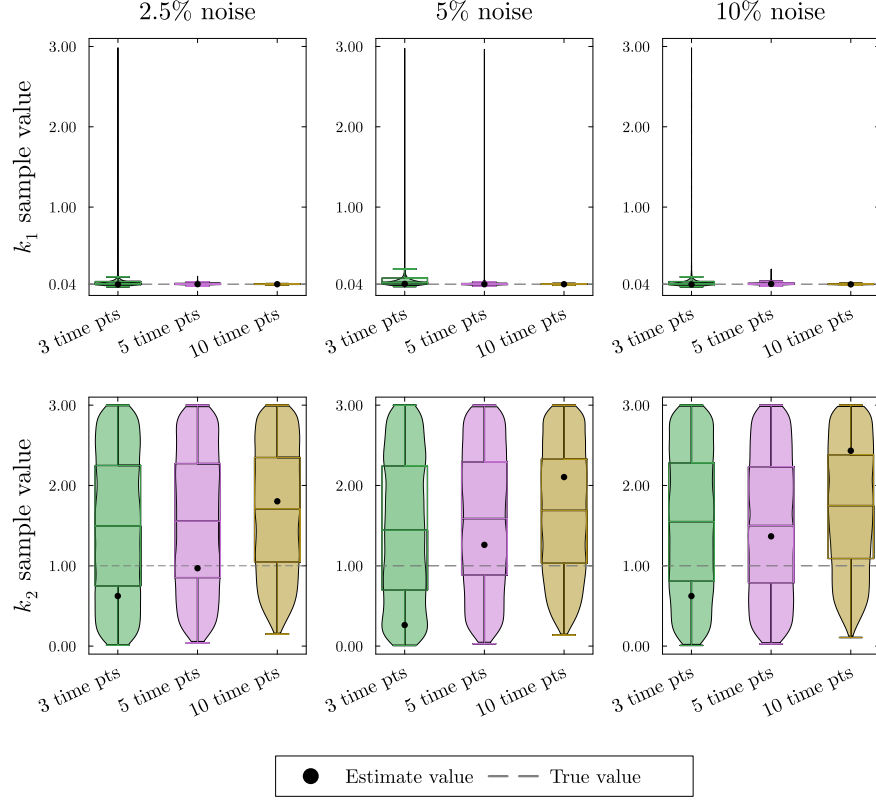

**Fig. 20** Violin and box plots for posterior distributions of  $k_1$  and  $k_2$  for the irreversible two-metabolite slow-fast system. The simulated data are taken from solutions of the system with parameters  $k_1 = 1/25$ ,  $\alpha_1 = 1/4$ ,  $k_2 = 1$ ,  $\alpha_2 = 2/5$  at 3, 5 or 10 equally distributed time points. At each time point, three noisy data points are simulated by adding random normally distributed noise to the true solutions with a standard deviation of 2.5, 5, or 10% of the true value. Since  $k_1$ , and  $k_2$  are turnover rates, we use the naive prior distributions  $k_1 \sim U(0, 3)$ ,  $k_2 \sim U(0, 3)$ . The mode of the posterior samples is taken as the estimated value. Outliers are excluded in the box plots

At the top of fig. 20, the estimates for  $k_1$  are very accurate and have extremely low uncertainty. With many experimental measurements throughout the decay of  $\bar{x}_1$ , we expected to get good estimates for  $k_1$ . Contrarily, we receive poor estimates for  $k_2$  with incredibly high uncertainty as shown at the bottom of fig. 20. The solution for  $\bar{x}_2$  is not sensitive to small changes in the large  $k_2$  value. With enough data points, Bayesian parameter estimation can rule out small values in  $k_2$  but cannot define a good range for the true value of the parameter.

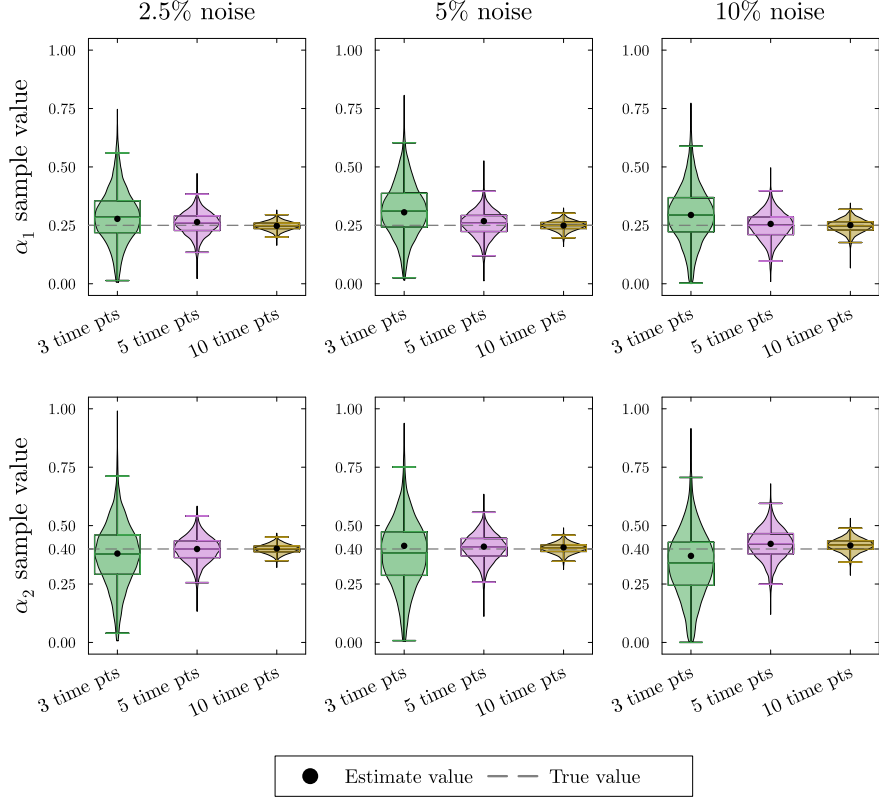

**Fig. 21** Violin and box plots for posterior distributions of  $\alpha_1$  and  $\alpha_2$  for the irreversible two-metabolite slow-fast system. The simulated data are taken from solutions of the system with parameters  $k_1 = 1/25$ ,  $\alpha_1 = 1/4$ ,  $k_2 = 1$ ,  $\alpha_2 = 2/5$  at 3, 5 or 10 equally distributed time points. At each time point, three noisy data points are simulated by adding random normally distributed noise to the true solutions with a standard deviation of 2.5, 5, or 10% of the true value. Since  $\alpha_1$  and  $\alpha_2$  are proportions, we use the natural naive prior distributions  $\alpha_1 \sim U(0, 1)$ ,  $\alpha_2 \sim U(0, 1)$ . The mode of the posterior samples is shown as a dot and is taken as the estimated value. Outliers are excluded in the box plots

As expected, in fig. 21, we see that increasing the number of time points produces a more accurate estimate value from the samples of the posterior distributions. We also note that the uncertainty in the estimation decreases with the increase in time points. Again with 10 time points and 2.5% noise, we receive the the best estimates with the least uncertainty for both  $\alpha_1$  and  $\alpha_2$ .

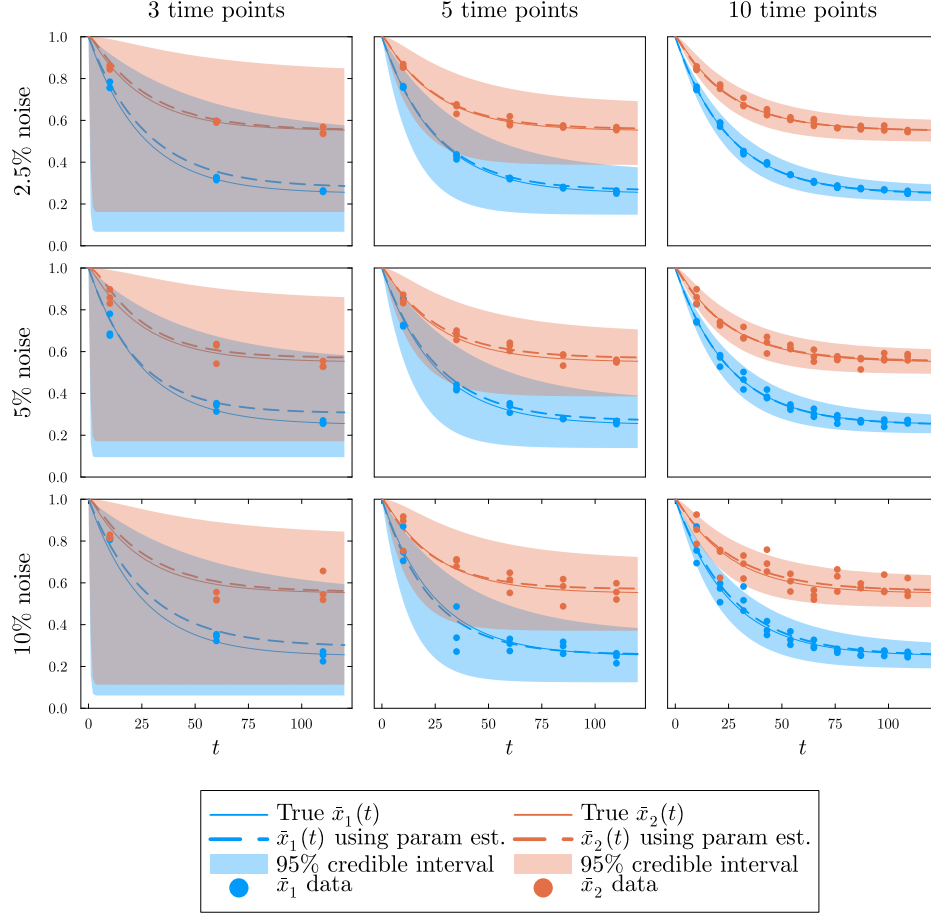

**Fig. 22** Comparing solutions using the values produced from Bayesian parameter estimation to the experimental data and true solutions for the irreversible two-metabolite slow-fast system. The simulated data are taken from solutions of the system with parameters  $k_1 = 1/25$ ,  $\alpha_1 = 1/4$ ,  $k_2 = 1$ ,  $\alpha_2 = 2/5$  at 3, 5 or 10 equally distributed time points. At each time point, three noisy data points are simulated by adding random normally distributed noise to the true solutions with a standard deviation of 2.5, 5, or 10% of the true value. The 95% credible interval was created by plotting the region between the solution with the 2.5% and the 97.5% quartiles of the posterior distributions of the parameters

In fig. 22, it appears that despite the inaccuracy and uncertainty in the estimate for  $k_2$ , the 95% credible interval for  $\bar{x}_2$  is a small interval around the true solution. This is because the solution for  $\bar{x}_2$  is not sensitive to small changes in the largest  $k$  value. Since the solution to  $\bar{x}_2$  doesn't change much with the changes in the value of  $k_2$ , a wide range of  $k_2$  values match the experimental measurements well.
